# Supplementary material for: Multiband effective bond-orbital model for nitride semiconductors with wurtzite structure
Source: arXiv:1001.3784 source file (2010-04-19)
Supplement: Supplementary file 1 [file supplementary_material.pdf]

# Supplementary material for “Multiband effective bond-orbital model for nitride semiconductors with wurtzite structure“

Daniel Mourad,* Stefan Barthel, and Gerd Czycholl
*Institute for Theoretical Physics, University of Bremen, D-28359 Bremen, Germany*
(Dated: March 16, 2010)

For an explanation of the physical meaning of the input parameters, we refer to Tab. I of the main text.

## I. EBOM WURTZIT-HAMILTONIAN

In this section, all matrix elements of the EBOM Hamiltonian for the hexagonal phase are analytically given as expressions with three-center integrals. As in the main text, the upper index in $E^{(k,l,m)}_{\alpha\alpha'}$ denotes $\mathbf{R}'-\mathbf{R}$ in units of half the lattice constants $a$ or $c$, respectively, so that

$$\mathbf{R}'-\mathbf{R}=\frac{ka}{2}\mathbf{e_x}+\frac{la}{2}\mathbf{e_y}+\frac{mc}{2}\mathbf{e_z}.$$

Furthermore, we abbreviate:

$$\begin{aligned}\xi &:= \frac{k_x a}{2},\\ \eta &:= \frac{k_y a}{2},\\ \rho &:= \frac{k_z c}{2}.\end{aligned}\tag{1}$$

In this notation, the matrix elements of Eq. (4) of the main text read as follows:

$$\begin{aligned}H_{ss}(\mathbf{k}) &= E_{ss}^{(0,0,0)}\\ &+ E_{ss}^{(\sqrt{3},1,0)}\cdot 4\cos(\xi\sqrt{3})\cos(\eta)\\ &+ E_{ss}^{(0,2,0)}\cdot 2\cos(2\eta)\\ &+ E_{ss}^{(0,0,2)}\cdot 2\cos(2\rho)\\ &+ E_{ss}^{(\sqrt{3},1,2)}\cdot 8\cos(\sqrt{3}\xi)\cos(\eta)\cos(2\rho)\\ &+ E_{ss}^{(0,2,2)}\cdot 4\cos(2\eta)\cos(2\rho)\\ &+ E_{ss}^{(0,0,4)}\cdot 2\cos(4\rho)\\ &+ E_{ss}^{(2\cdot\sqrt{3},2,0)}\cdot 2\cos(2\sqrt{3}\xi)\\ &+ E_{ss}^{(2\cdot\sqrt{3},2,0)}\cdot 4\cos(2\sqrt{3}\xi)\cos(2\eta)\\ &+ E_{ss}^{(\sqrt{3},3,0)}\cdot 4\cos(\sqrt{3}\xi)\cos(3\eta)\\ &+ E_{ss}(0,4,0)\cdot 2\cos(4\eta),\end{aligned}\tag{2}$$

$$\begin{aligned}H_{sx}(\mathbf{k}) &= E_{sx}^{(\sqrt{3},1,0)}\cdot 4i\sin(\xi\sqrt{3})\cos(\eta)\\ &+ E_{sx}^{(\sqrt{3},1,2)}\cdot 8i\sin(\xi\sqrt{3})\cos(\eta)\cos(2\rho)\\ &+ E_{sx}^{(2\cdot\sqrt{3},2,0)}\cdot 2i\sin(2\sqrt{3}\xi)\\ &+ E_{sx}^{(2\cdot\sqrt{3},2,0)}\cdot 4i\sin(2\sqrt{3}\xi)\cos(2\eta)\\ &+ E_{sx}^{(\sqrt{3},3,0)}\cdot 4i\sin(\sqrt{3}\xi)\cos(3\eta),\end{aligned}\tag{3}$$

$$\begin{aligned}H_{sy}(\mathbf{k}) &= E_{sy}^{(\sqrt{3},1,0)}\cdot 4i\sin(\eta)\cos(\xi\sqrt{3})\\ &+ E_{sy}^{(0,2,0)}\cdot 2i\sin(2\eta)\\ &+ E_{sy}^{(\sqrt{3},1,2)}\cdot 8i\cos(\xi\sqrt{3})\sin(\eta)\cos(2\rho)\\ &+ E_{sy}^{(0,2,2)}\cdot(4i\sin(2\eta)\cos(2\rho))\\ &+ E_{sy}^{(2\cdot\sqrt{3},2,0)}\cdot 4i\sin(2\eta)\cos(2\sqrt{3}\xi)\\ &+ E_{sy}^{(\sqrt{3},3,0)}\cdot 4i\cos(\sqrt{3}\xi)\sin(3\eta)\\ &+ E_{sy}^{(0,4,0)}\cdot 2i\sin(4\eta),\end{aligned}\tag{4}$$

$$\begin{aligned}H_{sz}(\mathbf{k}) &= E_{sz}^{(0,0,2)}\cdot(2i\sin(2\rho))\\ &+ E_{sz}^{(\sqrt{3},1,2)}\cdot 8i\cos(\xi\sqrt{3})\cos(\eta)\sin(2\rho)\\ &+ E_{sz}^{(0,2,2)}\cdot 4i\cos(2\eta)\sin(2\rho)\\ &+ E_{sz}^{(0,0,4)}\cdot 2i\sin(4\rho),\end{aligned}\tag{5}$$

$$\begin{aligned}H_{xx}(\mathbf{k}) &= E_{xx}^{(0,0,0)}\\ &+ E_{xx}^{(\sqrt{3},1,0)}\cdot 4\cos(\xi\sqrt{3})\cos(\eta)\\ &+ E_{xx}^{(0,2,0)}\cdot 2\cos(2\eta)\\ &+ E_{xx}^{(0,0,2)}\cdot 2\cos(2\rho)\\ &+ E_{xx}^{(\sqrt{3},1,2)}\cdot 8\cos(\sqrt{3}\xi)\cos(\eta)\cos(2\rho)\\ &+ E_{xx}^{(0,2,2)}\cdot 4\cos(2\eta)\cos(2\rho)\\ &+ E_{xx}^{(0,0,4)}\cdot 2\cos(4\rho)\\ &+ E_{xx}^{(2\cdot\sqrt{3},2,0)}\cdot 2\cos(2\sqrt{3}\xi)\\ &+ E_{xx}^{(2\cdot\sqrt{3},2,0)}\cdot 4\cos(2\sqrt{3}\xi)\cos(2\eta)\\ &+ E_{xx}^{(\sqrt{3},3,0)}\cdot 4\cos(\sqrt{3}\xi)\cos(3\eta)\\ &+ E_{xx}^{(0,4,0)}\cdot 2\cos(4\eta),\end{aligned}\tag{6}$$

$$\begin{aligned}H_{xy}(\mathbf{k}) &= E_{xy}^{(\sqrt{3},1,0)}\cdot 4\sin(\xi\sqrt{3})\sin(\eta)\\ &- E_{xy}^{(\sqrt{3},1,2)}\cdot 8\sin(\xi\sqrt{3})\sin(\eta)\cos(2\rho)\\ &- E_{xy}^{(2\cdot\sqrt{3},2,0)}\cdot 4\sin(2\sqrt{3}\xi)\sin(2\eta)\\ &- E_{xy}^{(\sqrt{3},3,0)}\cdot 4\sin(\sqrt{3}\xi)\sin(3\eta)\end{aligned}\tag{7}$$

$$H_{xz}(\mathbf{k}) = E_{xz}^{(\sqrt{3},1,2)}\cdot 8\sin(\xi\sqrt{3})\cos(\eta)\sin(2\rho),\tag{8}$$

$$H_{yy}(\mathbf{k}) = E_{yy}^{(0,0,0)}$$

$$
\begin{aligned}
&+ E_{yy}^{(\sqrt{3},1,0)} \cdot 4\cos(\xi\sqrt{3})\cos(\eta) \\
&+ E_{yy}^{(0,2,0)} \cdot 2\cos(2\eta) \\
&+ E_{yy}^{(0,0,2)} \cdot 2\cos(2\rho) \\
&+ E_{yy}^{(\sqrt{3},1,2)} \cdot 8\cos(\sqrt{3}\xi)\cos(\eta)\cos(2\rho) \\
&+ E_{yy}^{(0,2,2)} \cdot 4\cos(2\eta)\cos(2\rho) \\
&+ E_{yy}^{(0,0,4)} \cdot 2\cos(4\rho) \\
&+ E_{yy}^{(2\cdot\sqrt{3},2,0)} \cdot 2\cos(2\sqrt{3}\xi) \\
&+ E_{yy}^{(2\cdot\sqrt{3},2,0)} \cdot 4\cos(2\sqrt{3}\xi)\cos(2\eta) \\
&+ E_{yy}^{(\sqrt{3},3,0)} \cdot 4\cos(\sqrt{3}\xi)\cos(3\eta) \\
&+ E_{yy}^{(0,4,0)} \cdot 2\cos(4\eta), \qquad (9)
\end{aligned}
$$

$$
\begin{aligned}
H_{yz}(\mathbf{k}) &= E_{yz}^{(\sqrt{3},1,2)} \cdot 8\cos(\xi\sqrt{3})\sin(\eta)\sin(2\rho) \\
&- E_{yz}^{(0,2,2)} \cdot 4\sin(2\eta)\sin(2\rho), \qquad (10)
\end{aligned}
$$

$$
\begin{aligned}
H_{zz}(\mathbf{k}) &= E_{zz}^{(0,0,0)} \\
&+ E_{zz}^{(\sqrt{3},1,0)} \cdot 4\cos(\xi\sqrt{3})\cos(\eta) \\
&+ E_{zz}^{(0,2,0)} \cdot 2\cos(2\eta) \\
&+ E_{zz}^{(0,0,2)} \cdot 2\cos(2\rho) \\
&+ E_{zz}^{(\sqrt{3},1,2)} \cdot 8\cos(\sqrt{3}\xi)\cos(\eta)\cos(2\rho) \\
&+ E_{zz}^{(0,2,2)} \cdot 4\cos(2\eta)\cos(2\rho) \\
&+ E_{zz}^{(0,0,4)} \cdot 2\cos(4\rho) \\
&+ E_{zz} 2\cdot\sqrt{3}20 \cdot 2\cos(2\sqrt{3}\xi) \\
&+ E_{zz}^{(2\cdot\sqrt{3},2,0)} \cdot 4\cos(2\sqrt{3}\xi)\cos(2\eta) \\
&+ E_{zz}^{(\sqrt{3},3,0)} \cdot 4\cos(\sqrt{3}\xi)\cos(3\eta) \\
&+ E_{zz}^{(0,4,0)} \cdot 2\cos(4\eta), \qquad (11)
\end{aligned}
$$

## II. MODIFIED TWO-CENTER APPROXIMATION

In this section, we present the decomposition of the three-center integrals into two-center integrals. The subscript indices $\alpha, \beta, \gamma, \delta$, appearing in the two-center integrals

$$V_{\alpha\alpha'}(\beta)^{\gamma}(\delta) \qquad (12)$$

are denominated as follows: $\alpha = \{s, p\}$ describes the symmetry of the basis orbitals contributing to the three-center hopping integral (e.g. $s$- or $p$-like). $\gamma = \{\sigma, \pi\}$ stands for the symmetry type of the bond being established in standard molecular notation. $\delta = |\mathbf{R}' - \mathbf{R}|$ is the absolute value of the hopping distance between different lattice sites. As the hexagonal structure in is not invariant under cubic symmetry transformations (i.e. the crystal potential has lower symmetry than the basis orbitals), the two-center integrals must be distinguished additionally when a $p_z$- orbital is involved in the hopping. This is done by $\beta = \{a, c, aa, cc, ac\}$, which denotes if one or two of the involved basis orbitals lie in-plane $(a, aa)$ or off-plane $(c, cc)$. Mixtures are labeled as $(ac)$ and for $s$-like contributions in the hopping we drop this index, resulting in a single subscript. The prefactors occuring in the decomposition are given by the corresponding direction cosines. See Ref. 1 for further details.

$$
\begin{aligned}
E_{ss}^{(0,0,0)} &= V_{ss}^{\sigma}(0), \\
E_{xx}^{(0,0,0)} &= V_{pp}(aa)^{\pi}(0), \\
E_{yy}^{(0,0,0)} &= V_{pp}(aa)^{\pi}(0), \\
E_{zz}^{(0,0,0)} &= V_{pp}(cc)^{\pi}(0), \qquad (13)
\end{aligned}
$$

$$
\begin{aligned}
E_{ss}^{(\sqrt{3},1,0)} &= V_{ss}^{\sigma}(a), \\
E_{sx}^{(\sqrt{3},1,0)} &= \frac{\sqrt{3}}{2} \cdot V_{sp}(a)^{\sigma}(a), \\
E_{sy}^{(\sqrt{3},1,0)} &= \frac{1}{2} \cdot V_{sp}(a)^{\sigma}(a), \\
E_{xx}^{(\sqrt{3},1,0)} &= \frac{3}{4} \cdot V_{pp}(aa)^{\sigma}(a) + \frac{1}{4} \cdot V_{pp}(aa)^{\pi}(a), \\
E_{yy}^{(\sqrt{3},1,0)} &= \frac{1}{4} \cdot V_{pp}(aa)^{\sigma}(a) + \frac{3}{4} \cdot V_{pp}(aa)^{\pi}(a), \\
E_{zz}^{(\sqrt{3},1,0)} &= V_{pp}(cc)^{\pi}(a), \\
E_{xy}^{(\sqrt{3},1,0)} &= \frac{\sqrt{3}}{4} \cdot \Big(V_{pp}(aa)^{\sigma}(a) - V_{pp}(aa)^{\pi}(a)\Big), \qquad (14)
\end{aligned}
$$

$$
\begin{aligned}
E_{ss}^{(0,2,0)} &= V_{ss}^{\sigma}(a), \\
E_{sy}^{(0,2,0)} &= V_{sp}(a)^{\sigma}(a), \\
E_{xx}^{(0,2,0)} &= V_{pp}(aa)^{\pi}(a), \\
E_{yy}^{(0,2,0)} &= V_{pp}(aa)^{\sigma}(a), \\
E_{zz}^{(0,2,0)} &= V_{pp}(cc)^{\pi}(a), \qquad (15)
\end{aligned}
$$

$$
\begin{aligned}
E_{ss}^{(0,0,2)} &= V_{ss}^{\sigma}(c), \\
E_{sz}^{(0,0,2)} &= V_{sp}(c)^{\sigma}(c), \\
E_{xx}^{(0,0,2)} &= V_{pp}(aa)^{\pi}, \\
E_{yy}^{(0,0,2)} &= V_{pp}(aa)^{\pi}(c), \\
E_{zz}^{(0,0,2)} &= V_{pp}(cc)^{\sigma}(c), \qquad (16)
\end{aligned}
$$

$$
\begin{aligned}
E_{ss}^{(\sqrt{3},1,2)} &= V_{ss}^{\sigma}(\sqrt{a^2+c^2}), \\
E_{sx}^{(\sqrt{3},1,2)} &= V_{sp}(a)^{\sigma}(\sqrt{a^2+c^2}) \cdot \frac{\sqrt{3}a}{2\sqrt{a^2+c^2}}, \\
E_{sy}^{(\sqrt{3},1,2)} &= V_{sp}(a)^{\sigma}(\sqrt{a^2+c^2}) \cdot \frac{a}{\sqrt{a^2+c^2}}, \\
E_{sz}^{(\sqrt{3},1,2)} &= V_{sp}(c)^{\sigma}(\sqrt{a^2+c^2}) \cdot \frac{c}{\sqrt{a^2+c^2}} \qquad (17)
\end{aligned}
$$

$$
\begin{aligned}
E_{xx}^{(\sqrt{3},1,2)} &= \frac{1}{4(a^2+c^2)}\cdot\Big(3V_{pp}(aa)^{\sigma}(\sqrt{a^2+c^2})\cdot a^2,\\
&+ V_{pp}(aa)^{\pi}(\sqrt{a^2+c^2})\cdot a^2,\\
&+ 4V_{pp}(aa)^{\pi}(\sqrt{a^2+c^2})\cdot c^2\Big),\\
E_{yy}^{(\sqrt{3},1,2)} &= \frac{1}{4(a^2+c^2)}\cdot\Big(V_{pp}(aa)^{\sigma}(\sqrt{a^2+c^2})\cdot a^2,\\
&+ 3V_{pp}(aa)^{\pi}(\sqrt{a^2+c^2})\cdot a^2,\\
&+ 4V_{pp}(aa)^{\pi}(\sqrt{a^2+c^2})\cdot c^2\Big),\\
E_{zz}^{(\sqrt{3},1,2)} &= \frac{1}{a^2+c^2}\cdot\Big(V_{pp}(cc)^{\sigma}(\sqrt{a^2+c^2})\cdot c^2,\\
&+ V_{pp}^{\pi}(cc)(\sqrt{a^2+c^2})\cdot a^2\Big),\\
E_{xy}^{(\sqrt{3},1,2)} &= \frac{\sqrt{3}a^2}{4(a^2+c^2)}\cdot\Big(V_{pp}(aa)^{\sigma}(\sqrt{a^2+c^2}),\\
&- V_{pp}(aa)^{\pi}(\sqrt{a^2+c^2})\Big),\\
E_{xz}^{(\sqrt{3},1,2)} &= \frac{\sqrt{3}ac}{2(a^2+c^2)}\cdot\Big(V_{pp}(ac)^{\sigma}(\sqrt{a^2+c^2})\\
&- V_{pp}(ac)^{\pi}(\sqrt{a^2+c^2})\Big),\\
E_{yz}^{(\sqrt{3},1,2)} &= \frac{ac}{2(a^2+c^2)}\cdot\Big(V_{pp}(ac)^{\sigma}(\sqrt{a^2+c^2}),\\
&- V_{pp}(ac)^{\pi}(\sqrt{a^2+c^2})\Big) \qquad (18)
\end{aligned}
$$

$$
\begin{aligned}
E_{ss}^{(0,2,2)} &= V_{ss}^{\sigma}(\sqrt{a^2+c^2}),\\
E_{sy}^{(0,2,2)} &= V_{sp}(a)^{\sigma}(\sqrt{a^2+c^2})\cdot\frac{a}{\sqrt{a^2+c^2}},\\
E_{sz}^{(0,2,2)} &= V_{sp}(c)^{\sigma}(\sqrt{a^2+c^2})\cdot\frac{c}{\sqrt{a^2+c^2}},\\
E_{xx}^{(0,2,2)} &= V_{pp}(aa)^{\pi}(\sqrt{a^2+c^2}),\\
E_{yy}^{(0,2,2)} &= \Big(V_{pp}(aa)(\sqrt{a^2+c^2})^{\sigma}\cdot a^2,\\
&+ V_{pp}(aa)(\sqrt{a^2+c^2})^{\pi}\cdot c^2\Big)\frac{1}{a^2+c^2},\\
E_{zz}^{(0,2,2)} &= \Big(V_{pp}(cc)^{\sigma}(\sqrt{a^2+c^2})\cdot c^2,\\
&+ V_{pp}(cc)^{\pi}(\sqrt{a^2+c^2})\cdot a^2\Big)\frac{1}{a^2+c^2},\\
E_{yz}^{(0,2,2)} &= \Big(V_{pp}(ac)^{\sigma}(\sqrt{a^2+c^2}),\\
&- V_{pp}(ac)^{\pi}(\sqrt{a^2+c^2})\Big)\frac{ac}{a^2+c^2}, \qquad (19)
\end{aligned}
$$

$$
\begin{aligned}
E_{ss}^{(0,0,4)} &= V_{ss}^{\sigma}(2c),\\
E_{sz}^{(0,0,4)} &= V_{sp}(c)^{\sigma}(2c),\\
E_{xx}^{(0,0,4)} &= V_{pp}(aa)^{\pi}(2c),\\
E_{yy}^{(0,0,4)} &= V_{pp}(aa)^{\pi}(2c),\\
E_{zz}^{(0,0,4)} &= V_{pp}(cc)^{\sigma}(2c), \qquad (20)
\end{aligned}
$$

$$
\begin{aligned}
E_{ss}^{(2\cdot\sqrt{3},0,0)} &= V_{ss}^{\sigma}(\sqrt{3}a),\\
E_{sx}^{(2\cdot\sqrt{3},0,0)} &= V_{sp}(a)^{\sigma}(\sqrt{3}a),\\
E_{xx}^{(2\cdot\sqrt{3},0,0)} &= V_{pp}(aa)^{\sigma}(\sqrt{3}a),\\
E_{yy}^{(2\cdot\sqrt{3},0,0)} &= V_{pp}(aa)^{\pi}(\sqrt{3}a),\\
E_{zz}^{(2\cdot\sqrt{3},0,0)} &= V_{pp}(cc)^{\pi}(\sqrt{3}a),\\
E_{ss}^{(2\cdot\sqrt{3},2,0)} &= V_{ss}^{\sigma}(2a), \qquad (21)
\end{aligned}
$$

$$
\begin{aligned}
E_{sx}^{(2\cdot\sqrt{3},2,0)} &= \frac{\sqrt{3}}{2}\cdot V_{sp}(a)^{\sigma}(2a),\\
E_{sy}^{(2\cdot\sqrt{3},2,0)} &= \frac{1}{2}\cdot V_{sp}(a)^{\sigma}(2a),\\
E_{xx}^{(2\cdot\sqrt{3},2,0)} &= \frac{3}{4}\cdot V_{pp}(aa)^{\sigma}(2a)+\frac{1}{4}\cdot V_{pp}(aa)^{\pi}(2a),\\
E_{yy}^{(2\cdot\sqrt{3},2,0)} &= \frac{1}{4}\cdot V_{pp}(aa)^{\sigma}(2a)+\frac{3}{4}\cdot V_{pp}(aa)^{\pi}(2a),\\
E_{zz}^{(2\cdot\sqrt{3},2,0)} &= V_{pp}(cc)^{\pi}(2a),\\
E_{xy}^{(2\cdot\sqrt{3},2,0)} &= \frac{\sqrt{3}}{4}\cdot\Big(V_{pp}(aa)^{\sigma}(2a),\\
&- V_{pp}(aa)^{\pi}(2a)\Big), \qquad (22)
\end{aligned}
$$

$$
\begin{aligned}
E_{ss}^{(\sqrt{3},3,0)} &= V_{ss}^{\sigma}(\sqrt{3}a),\\
E_{sx}^{(\sqrt{3},3,0)} &= \frac{1}{2}\cdot V_{sp}(a)^{\sigma}(\sqrt{3}a),\\
E_{sy}^{(\sqrt{3},3,0)} &= \frac{\sqrt{3}}{2}\cdot V_{sp}(a)^{\sigma}(\sqrt{3}a),\\
E_{xx}^{(\sqrt{3},3,0)} &= \frac{1}{4}\cdot V_{pp}(aa)^{\sigma}(\sqrt{3}a)+\frac{3}{4}\cdot V_{pp}(aa)^{\pi}(\sqrt{3}a),\\
E_{yy}^{(\sqrt{3},3,0)} &= \frac{3}{4}\cdot V_{pp}(aa)^{\sigma}(\sqrt{3}a)+\frac{1}{4}\cdot V_{pp}(aa)^{\pi}(\sqrt{3}a)\\
E_{zz}^{(\sqrt{3},3,0)} &= V_{pp}(cc)^{\pi}(\sqrt{3}a),\\
E_{xy}^{(\sqrt{3},3,0)} &= \frac{\sqrt{3}}{4}\cdot\Big(V_{pp}(aa)^{\sigma}(\sqrt{3}a),\\
&- V_{pp}(aa)^{\pi}(\sqrt{3}a)\Big), \qquad (23)
\end{aligned}
$$

$$
\begin{aligned}
E_{ss}^{(0,4,0)} &= V_{ss}^{\sigma}(2a),\\
E_{sy}^{(0,4,0)} &= V_{sp}(a)^{\sigma}(2a),\\
E_{xx}^{(0,4,0)} &= V_{pp}(aa)\pi(2a),\\
E_{yy}^{(0,4,0)} &= V_{pp}(aa)^{\sigma}(2a),\\
E_{zz}^{(0,4,0)} &= V_{pp}(cc)^{\pi}(2a). \qquad (24)
\end{aligned}
$$

## III. COMPARISON TO $\mathbf{k}\cdot\mathbf{p}$-REPRESENTATION

In order to have the complete parametrization included in this supplementary material, we repeat here the results of the comparison to the $\mathbf{k}\cdot\mathbf{p}$-representation of Appendix A of the main text:

$$P_{\parallel,\perp} = \sqrt{\frac{\hbar^2}{2m_0}E_p^{\parallel,\perp}} \tag{25}$$

$$P_{\parallel}^2 = \frac{\hbar^2}{2m_0}\left(\frac{m_0}{m_e^{\parallel}}-1\right)\frac{3E_g(\Delta_{so}+E_g)+\Delta_{cr}(2\Delta_{so}+3E_g)}{2\Delta_{so}+3E_g}, \tag{26}$$

$$P_{\perp}^2 = \frac{\hbar^2}{2m_0}\left(\frac{m_0}{m_e^{\perp}}-1\right)E_g\frac{[3E_g(\Delta_{so}+E_g)+\Delta_{cr}(2\Delta_{so}+3E_g)]}{\Delta_{cr}\Delta_{so}+3\Delta_{cr}E_g+2\Delta_{so}E_g+3E_g^2}. \tag{27}$$

$$\begin{aligned}
\frac{\hbar}{2m_e^{\parallel}}-\frac{P_{\parallel}^2}{E_g} &= \left(-4E_{ss}^{(\sqrt{3},1,2)}-2E_{ss}^{(0,2,2)}-4E_{ss}^{(0,0,4)}-E_{ss}^{(0,0,2)}\right)\cdot c^2,\\
\frac{\hbar}{2m_e^{\perp}}-\frac{P_{\perp}^2}{E_g} &= \left(-E_{ss}^{(0,2,0)}-E_{ss}^{(\sqrt{3},1,2)}-2E_{ss}^{(0,2,2)}-\frac{1}{2}E_{ss}^{(\sqrt{3},1,0)}-4E_{ss}^{(0,4,0)}-\frac{9}{2}E_{ss}^{(\sqrt{3},3,0)}-2E_{ss}^{(2\sqrt{3},2,0)}\right)\cdot a^2,\\
\frac{\hbar}{2m_e^{\perp}}-\frac{P_{\perp}^2}{E_g} &= \left(-\frac{3}{2}E_{ss}^{(\sqrt{3},1,0)}-3E_{ss}^{(\sqrt{3},1,2)}-\frac{3}{2}E_{ss}^{(\sqrt{3},3,0)}-6E_{ss}^{(2\sqrt{3},2,0)}-3E_{ss}^{(2\sqrt{3},0,0)}\right)\cdot a^2,\\
iP_{\perp} &= \left(2iE_{sx}^{(\sqrt{3},1,0)}+4iE_{sx}^{(\sqrt{3},1,2)}+2iE_{sx}^{(2\sqrt{3},0,0)}+4iE_{sx}^{(2\sqrt{3},2,0)}+2iE_{sx}^{(\sqrt{3},3,0)}\right)\cdot a\sqrt{3},\\
iP_{\perp} &= \left(2iE_{sy}^{(\sqrt{3},1,0)}+2iE_{sy}^{(0,2,0)}+4iE_{sy}^{(\sqrt{3},1,2)}+4iE_{sy}^{(0,2,2)}+4iE_{sy}^{(2\sqrt{3},2,0)}+6iE_{sy}^{(\sqrt{3},3,0)}+4iE_{sy}^{(0,4,0)}\right)\cdot a,\\
iP_{\parallel} &= \left(2iE_{sz}^{(0,0,2)}+8iE_{sz}^{(\sqrt{3},1,2)}+4iE_{sz}^{(0,2,2)}+4iE_{sz}^{(0,0,4)}\right)\cdot c,\\
A_2+A_4+A_5+\frac{P_{\parallel}^2}{E_g} &= \left(-\frac{3}{2}E_{xx}^{(\sqrt{3},1,0)}-3E_{xx}^{(\sqrt{3},1,2)}-\frac{3}{2}E_{xx}^{(\sqrt{3},3,0)}-6E_{xx}^{(2\sqrt{3},2,0)}-3E_{xx}^{(2\sqrt{3},0,0)}\right)\cdot a^2,\\
A_2+A_4-A_5 &= \left(-E_{xx}^{(0,2,0)}-E_{xx}^{(\sqrt{3},1,2)}-2E_{xx}^{(0,2,2)}-\frac{1}{2}E_{xx}^{(\sqrt{3},1,0)}-4E_{xx}^{(0,4,0)}-\frac{9}{2}E_{xx}^{(\sqrt{3},3,0)}-2E_{xx}^{(2\sqrt{3},2,0)}\right)\cdot a^2,\\
A_1+A_3 &= \left(-4E_{xx}^{(\sqrt{3},1,2)}-2E_{xx}^{(0,2,2)}-4E_{xx}^{(0,0,4)}-E_{xx}^{(0,0,2)}\right)\cdot c^2,\\
2A_5+\frac{P_{\parallel}^2}{E_g} &= \left(-E_{xy}^{(\sqrt{3},1,0)}-2E_{xy}^{(\sqrt{3},1,2)}-4E_{xy}^{(2\sqrt{3},2,0)}-3E_{xy}^{(\sqrt{3},3,0)}\right)\cdot a^2\sqrt{3},\\
\sqrt{2}A_6+\frac{P_{\parallel}P_{\perp}}{E_g} &= -4E_{xz}^{(\sqrt{3},1,2)}\cdot a\sqrt{3}c,\\
A_2+A_4-A_5 &= \left(-\frac{3}{2}E_{yy}^{(\sqrt{3},1,0)}-3E_{yy}^{(\sqrt{3},1,2)}-\frac{3}{2}E_{yy}^{(\sqrt{3},3,0)}-6E_{yy}^{(2\sqrt{3},2,0)}-3E_{yy}^{(2\sqrt{3},0,0)}\right)\cdot a^2,\\
A_2+A_4+A_5+\frac{P_{\parallel}^2}{E_g} &= \left(-E_{yy}^{(0,2,0)}-E_{yy}^{(\sqrt{3},1,2)}-2E_{yy}^{(0,2,2)}-\frac{1}{2}E_{yy}^{(\sqrt{3},1,0)}-4E_{yy}^{(0,4,0)}-\frac{9}{2}E_{yy}^{(\sqrt{3},3,0)}-2E_{yy}^{(2\sqrt{3},2,0)}\right)\cdot a^2,\\
A_1+A_3 &= \left(-4E_{yy}^{(\sqrt{3},1,2)}-2E_{yy}^{(0,2,2)}-4E_{yy}^{(0,0,4)}-E_{yy}^{(0,0,2)}\right)\cdot c^2,\\
\sqrt{2}A_6+\frac{P_{\parallel}P_{\perp}}{E_g} &= \left(-4E_{yz}^{(\sqrt{3},1,2)}-4E_{yz}^{(0,2,2)}\right)\cdot ac,\\
A_2 &= \left(-\frac{3}{2}E_{zz}^{(\sqrt{3},1,0)}-3E_{zz}^{(\sqrt{3},1,2)}-\frac{3}{2}E_{zz}^{(\sqrt{3},3,0)}-6E_{zz}^{(2\sqrt{3},2,0)}-3E_{zz}^{(2\sqrt{3},0,0)}\right)\cdot a^2,\\
A_2 &= \left(-E_{zz}^{(0,2,0)}-E_{zz}^{(\sqrt{3},1,2)}-2E_{zz}^{(0,2,2)}-\frac{1}{2}E_{zz}^{(\sqrt{3},1,0)}-4E_{zz}^{(0,4,0)}-\frac{9}{2}E_{zz}^{(\sqrt{3},3,0)}-2E_{zz}^{(2\sqrt{3},2,0)}\right)\cdot a^2,\\
A_1+\frac{P_{\perp}^2}{E_g} &= \left(-4E_{zz}^{(\sqrt{3},1,2)}-2E_{zz}^{(0,2,2)}-4E_{zz}^{(0,0,4)}-E_{zz}^{(0,0,2)}\right)\cdot c^2.
\end{aligned} \tag{28}$$

## IV. PSEUDOCODE DESCRIPTION

We already pointed out that the solution of the above given system of equations (which includes the analytical solution of the bulk secular equation, Eq. (3) of the main text, for the critical **k**-values of Tab. I of the main text) for the two-center integrals, which links them to known band structure parameters, leads to very unhandy expressions. So the explicit solution is given as ASCII-code in Ref. 2. The first paragraph in the file corresponds to the solution for the $G_0W_0$ parameters and the second one to the corrected $G_0W_0$ parameters (see main text for further details). The decomposition into two-center integrals as MATLAB-compatible pseudocode is listed in the same order as presented here directly in the last paragraph. In the following, we will give the pseudocode notation (left side) of the physical quantities (right side). The effective electron masses, valence band parameters, spin-orbit and crystal field splittings are given by:

$$\begin{aligned} \text{me\_z} &:= m_e^{\parallel}, \\ \text{me\_t} &:= m_e^{\perp}, \\ \text{A\_1} &:= A_1, \\ \text{A\_2} &:= A_2, \\ \ldots &:= \ldots, \\ \text{A\_6} &:= A_6, \\ \text{Delta\_so} &:= \Delta_{so}, \\ \text{Delta\_cr} &:= \Delta_{cr}. \end{aligned}$$

The eigenenergies for the high-symmetry points are given by:

$$\begin{aligned} \text{E\_g} &:= \Gamma_1^c - \Gamma_6^v, \\ \text{Es\_0} &:= \Gamma_1^c, \\ \text{Ep\_0} &:= \Gamma_6^v - \left(\Delta_{cr} + \frac{\Delta_{so}}{3}\right), \end{aligned}$$

$$\tilde{\text{E}}\text{p\_0} := \Gamma_6^v - \frac{1}{2}\left(\Delta_{cr} - \frac{\Delta_{so}}{3} + \sqrt{\left(\Delta_{cr} - \frac{\Delta_{so}}{3}\right)^2 + 8\left(\frac{\Delta_{so}}{3}\right)^2}\right),$$

$$\begin{aligned} \text{Ep\_A1} &:= A_{1,3}^c, \\ \text{Ep\_A2} &:= A_{5,6}^v, \\ \text{Ep\_A3} &:= A_{1,3}^v, \\ \text{Ep\_L1} &:= L_{1,3}^c, \\ \text{Ep\_L3} &:= L_{1,3}^v, \\ \text{Ep\_L2} &:= L_{2,4}^v, \\ \text{Ep\_L4} &:= L_{1,3}^{v*}, \\ \text{Ep\_M1} &:= M_1^c, \\ \text{Ep\_M2} &:= M_4^v, \\ \text{Ep\_M4} &:= M_3^v, \\ \text{Ep\_M3} &:= M_1^v, \\ \text{Ep\_H1} &:= H_3^c, \\ \text{Ep\_H2} &:= H_3^v, \\ \text{Ep\_H3} &:= H_3^{v*}. \end{aligned} \tag{29}$$

The only difference is that for AlN one has to use Ẽp_0 instead of Ep_0. The latter only holds for the GaN and InN material systems, because the order of the valence bands changes in respect to AlN. The Kane parameters are finally given by:

$$\begin{aligned} \text{P\_z} &:= P_{\parallel}, \\ \text{P\_t} &:= P_{\perp}. \end{aligned}$$

* Electronic address: dmourad@itp.uni-bremen.de

[1] J. C. Slater and G. F. Koster, Phys. Rev. **94**, 1498 (1954).
[2] See EPAPS Document No. for the explicit solution of the resulting system of equations.
